# Supplementary material for: Hot-carrier transfer across a nanoparticle-molecule junction: The importance of orbital hybridization and level alignment
Source: arXiv:2206.05027 ancillary file (2022-06-10)
Supplement: Supplementary file 1 [file Supplementary_Information.pdf]

# Supplementary Material

## Hot-carrier transfer across a nanoparticle-molecule junction: The importance of orbital hybridization and level alignment

Jakub Fojt, Tuomas P. Rossi, and Paul Erhart

## Contents

**Figures** **2**

S1. Absorption spectrum of free CO molecule along its bond axis . . . 2
S2. Frequency and width of $Ag_{201}$ LSP . . . 2
S3. Binding energies of CO + $Ag_{201}$ under constrained relaxation . . . 3
S4. Carrier generation on the molecule after plasmon decay . . . 4
S5. Projected density of states for the molecule, in the combined system . . . 5
S6. Decomposition of electrons generated on the molecule in electrons and holes, depending on pulse frequency . . . 6
S7. Density of states of $Ag_{201}$, $Au_{201}$, and $Cu_{201}$ . . . 7
S8. Binding energies of the combined CO + NP system as a function of site and distance . . . 7
S9. Pulse-frequency dependence of the electron generation in CO . . . 8
S10. Alternative formulations of electron distribution in molecule after plasmon decay . . . 9
S11. Level alignment between the projected densities of state of the NP and molecule for $Ag_{201}$ 10
S12. Level alignment between the projected densities of state of the NP and molecule for $Au_{201}$ and $Cu_{201}$ . . . 11
S13. Carrier generation depending on occupation number smearing . . . 11

# Figures

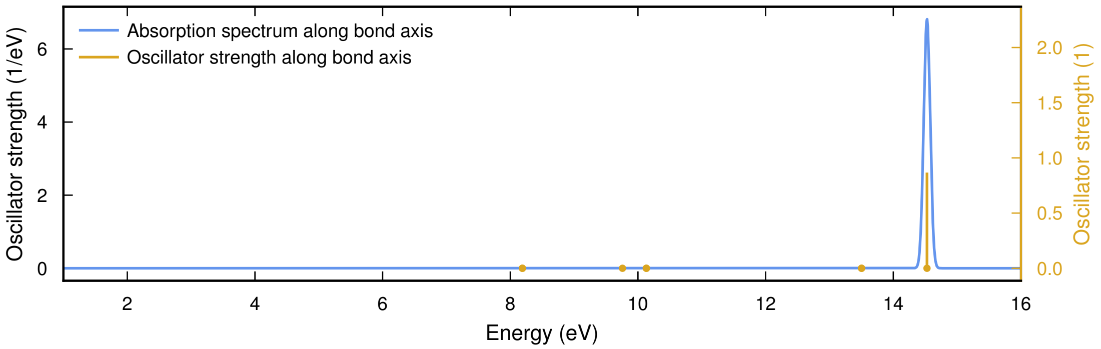


Figure S1: **Absorption spectrum of free CO molecule along its bond axis.** The free CO molecule (bond length 1.144 Å) has its first excited state at 8.19 eV. This is an optically dark state that corresponds to the HOMO-LUMO transition. The first bright state is 14.53 eV. The transitions were obtained by linear response TDDFT calculations in GPAW with the xc-functional PBE.

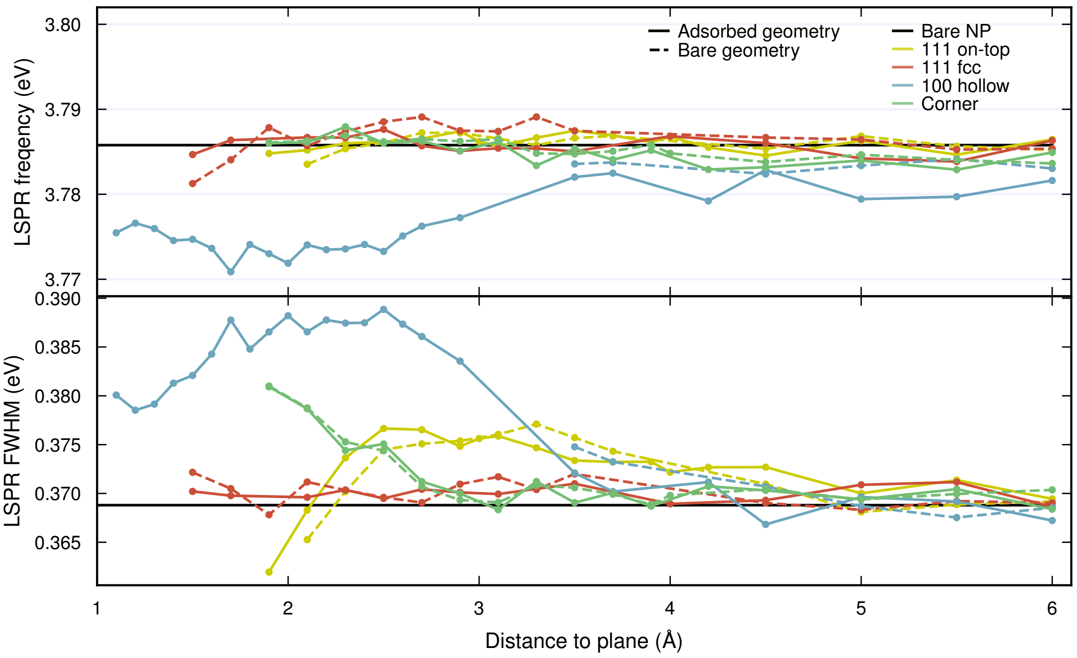


Figure S2: **Frequency and width of $Ag_{201}$ LSP.** The bare NP has a LSP frequency close to 3.8 eV (determined by fitting a Lorentizan function to the spectrum). Adding the CO molecule shifts the LSP frequency by less than 15 meV for the 100 hollow site, and less than 5 meV for the other sites.

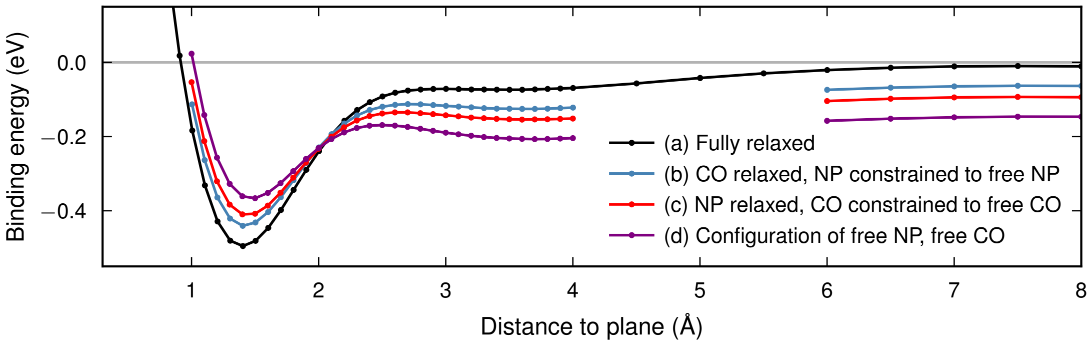


Figure S3: **Binding energies of CO + $Ag_{201}$ under constrained relaxation.** The binding energy is defined $E^{(\mathrm{site})}_{\mathrm{bind}}(d) = E^{(\mathrm{site})}(d) - E^{(\mathrm{site})}_{\mathrm{NP}} - E^{(\mathrm{site})}_{\mathrm{mol}}$ where $E^{(\mathrm{site})}_{\mathrm{NP}}$ ($E^{(\mathrm{site})}_{\mathrm{mol}}$) is the energy of the system, in its adsorbed configuration, without the molecule (NP). Binding energies are computed by rigidly displacing the CO along a line from the (111) on-top site of the NP, from 4 different starting positions. The starting positions are:

(a) The combined system (NP and CO) is fully relaxed in the adsorption minimum (same as in Figure S8.

(b) The combined system is relaxed with a constraint: all Ag atoms are fixed in the positions of the free NP.

(c) The combined system is relaxed with a constraint: the CO bond length is fixed to the bond length of the free molecule.

(d) The combined system is not relaxed. The configuration of a free NP and free molecule are used.

Of the 4 options fully relaxing the system (a) gives the lowest energies close to the adsorption minimum, but the highest in the long-distance limit, which is expected. Taking the free NP and free molecule configurations (d) gives the highest energies close to the adsorption minimum and the lowest in the long-distance limit. The relaxation of the molecule only (b; the bond length increases compared to the bond length of free CO) and of the NP only (c; which manifests itself as distortion of the NP surface close to the CO) contribute roughly equally to the energies. In principle finding a minimum energy path over the entire range of distances can be done, by performing a constrained relaxation at every distance. Such a calculation would yield a curve that is at every distance lower in energy than any other curve, effectively widening the adsorption minimum. Note that as the reference $E^{(\mathrm{site})}_{\mathrm{NP}}$, and $E^{(\mathrm{site})}_{\mathrm{mol}}$ are taken for the fully relaxed configurations binding energies at long distances are negative for options (b-d); this is the expected behavior for our definition of binding energy.

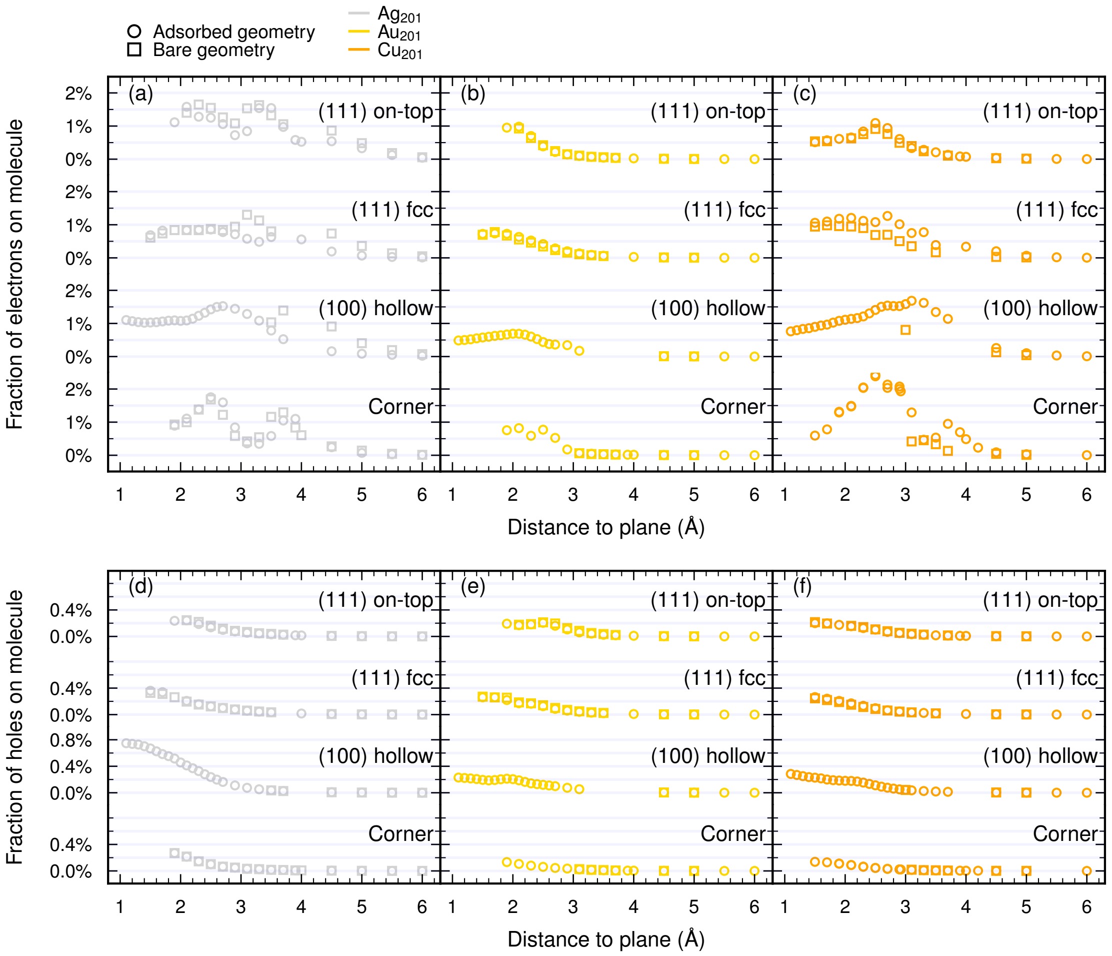


Figure S4: **Carrier generation on the molecule after plasmon decay.** Electrons (a-c) and holes (d-f) generated in $Ag_{201}$ (a, d), $Au_{201}$ (b, e), $Cu_{201}$ (c, f) for the considered sites, distances, and geometrical configurations. "Adsorbed geometry" refers to the combined system that has been relaxed in the adsorption minimum, and the molecule then shifted. "Bare geometry" refers to the NP being configured as the free NP and the CO with the bond length of the free CO molecule. For the two types of geometries, the curves are similar for the electrons (with the exception of a few features), and practically identical for the holes. The differences for the electrons are explained by the shift in the CO LUMO orbital due to changing bond length, which affects the resonance condition (Figure S11). Pulse frequencies are 3.8 eV (Ag), 2.5 eV (Au) and 2.7 eV (Cu).

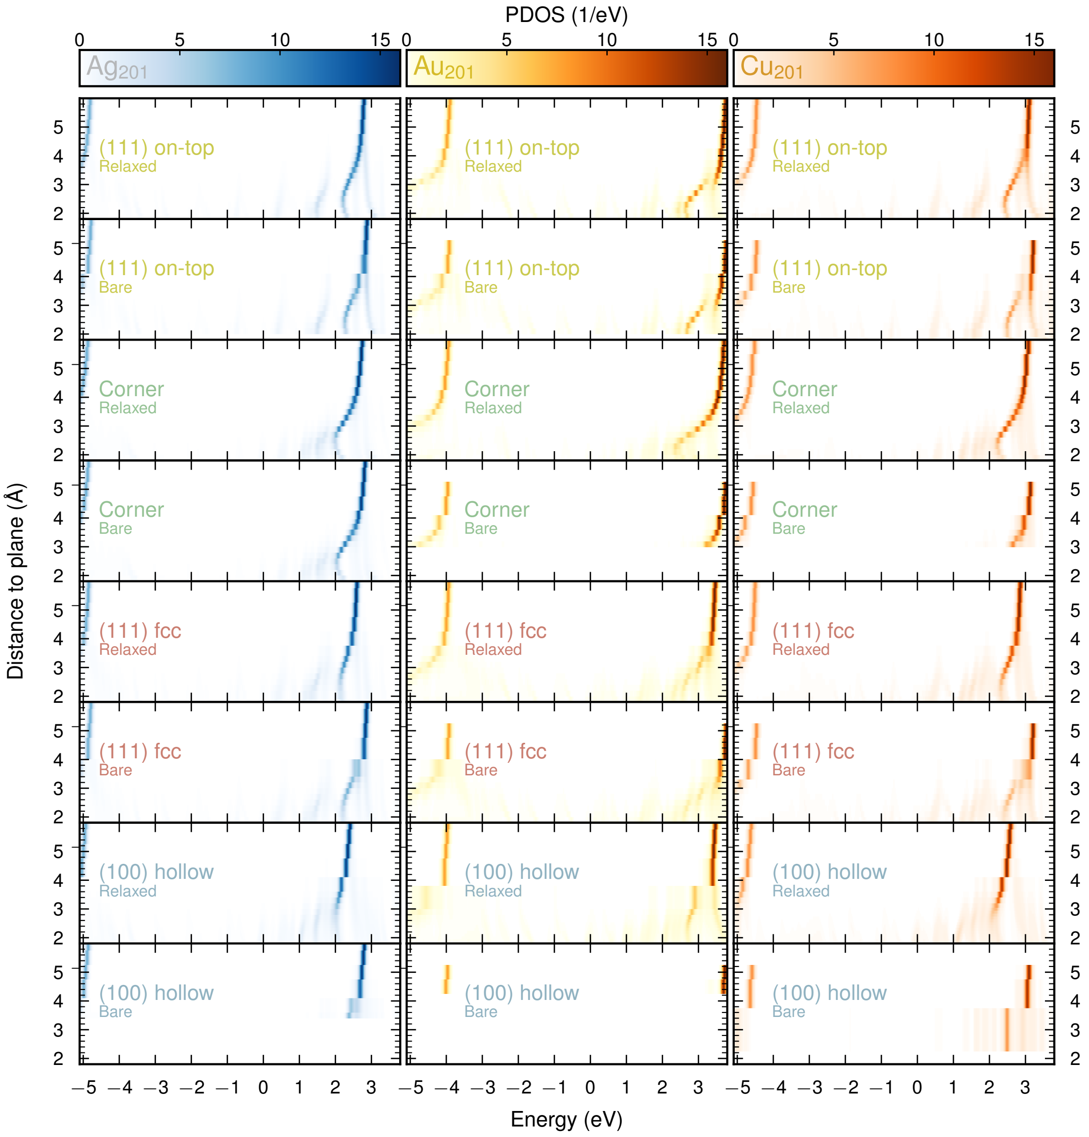


Figure S5: **Projected density of states for the molecule, in the combined system.** As the molecule is brought closer to the NP, the HOMO and LUMO orbitals shift to lower energies (distance 4-6 Å) and hybridize, splitting up into several branches (distances smaller than 4 Å).

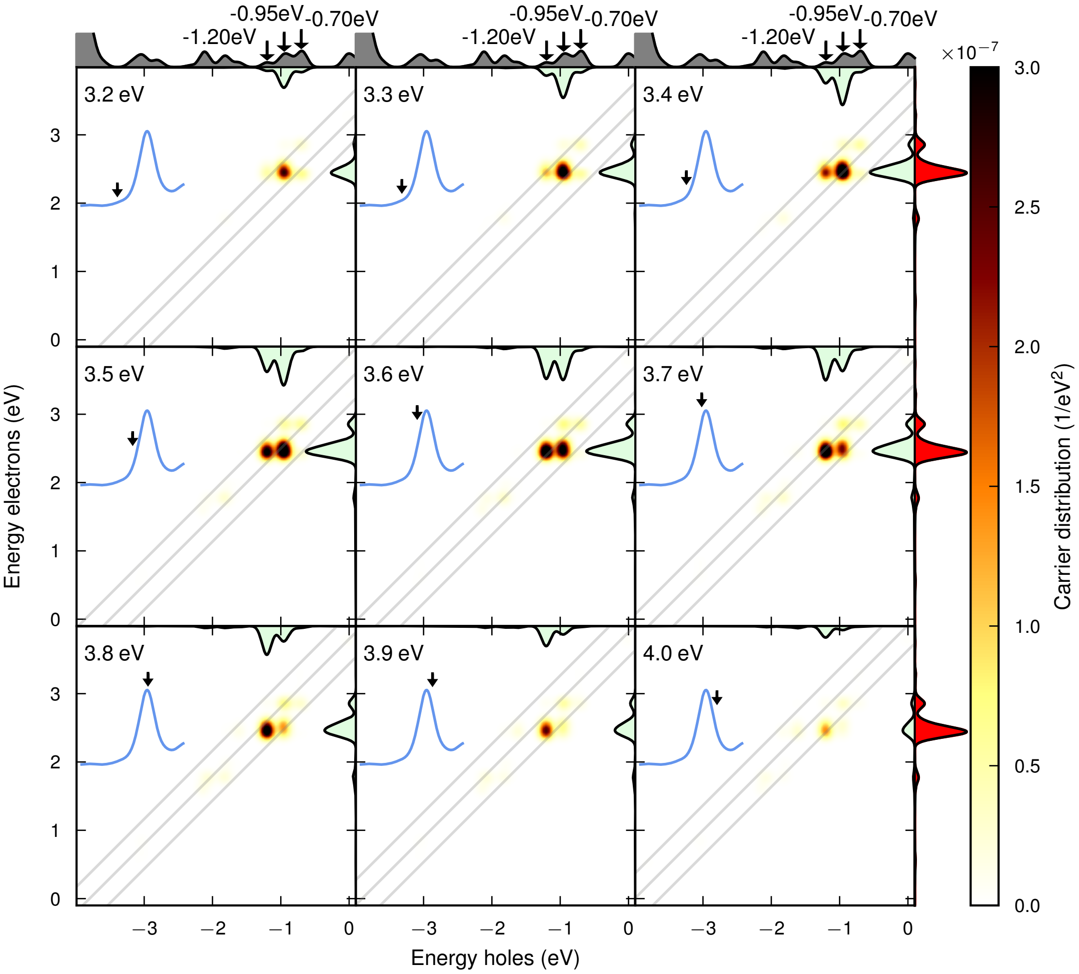


Figure S6: **Decomposition of electrons generated on the molecule in electrons and holes, depending on pulse frequency.** The quantity $\sum_{ia} M_{ia} w_{aa'}^{(\mathrm{mol})} \delta(\varepsilon - \varepsilon_a)\delta(\varepsilon - \varepsilon_i)$ where $M_{ia} = \sum_{a'}^{f_i > f_a, f_i > f_{a'}} (q_{ia} q_{ia'} + p_{ia} p_{ia'})$ shows a map between holes (in the combined system NP+CO) and electrons in the CO molecule, for a particular geometry ($Ag_{201}$ (111) on-top distance 3.3 Å). The map with hole/electron dependence integrated out ($\sum_{ia} M_{ia} w_{aa'}^{(\mathrm{mol})} \delta(\varepsilon - \varepsilon_a) / \sum_{ia} M_{ia} w_{aa'}^{(\mathrm{mol})} \delta(\varepsilon - \varepsilon_i)$) is shown on the inner axes in a fixed scale. DOS of the combined system and PDOS of the molecule are shown on the outer axes. The inset of the optical spectrum shows the pulse frequency used. The electron transfer involves primarily occupied states at three energies ($-1.2$, $-0.95$ and $-0.7$ eV) and unoccupied states in the molecule at three levels. As involved states need to be resonant ($\varepsilon_a - \varepsilon_i = \hbar\omega_{\mathrm{pulse}}$, indicated by the middle diagonal line, while the outer diagonal lines indicate the half-width at half-maximum of the pulse 0.37 eV) the contribution of each state varies with pulse frequency. Maximum electron transfer is achieved at 3.5-3.6 eV, slightly off the LSP resonance, when the states at $-1.2$ and $-0.95$ eV are resonant with the main LUMO branch. The former states occupied states are thus interacting more strongly with the transfer to the LUMO than the states at $-0.7$ eV.

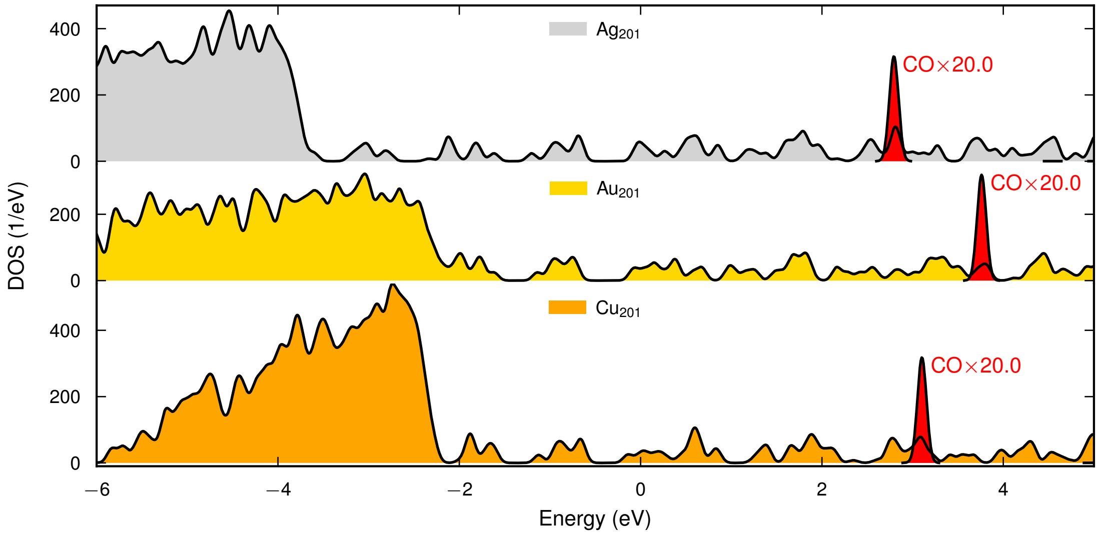


Figure S7: **Density of states of $Ag_{201}$, $Au_{201}$, and $Cu_{201}$.** The DOS is shown relative to Fermi level, and the PDOS of the molecule at far distances is included in the figure, showing its alignment to the different metals.

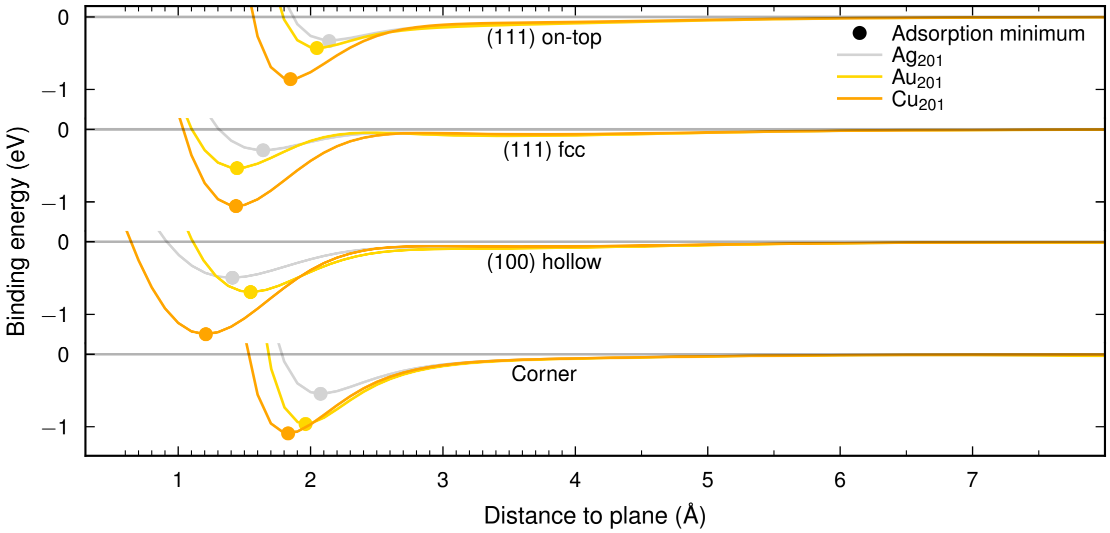


Figure S8: **Binding energies of the combined CO + NP system as a function of site and distance.** Energies are computed in VASP using the vdW-cx-df xc-functional. The molecule is rigidly displaced from its adsorption minimum without allowing neither the bond length nor the NP to relax. The binding energy is defined $E^{(\mathrm{site})}_{\mathrm{bind}}(d) = E^{(\mathrm{site})}(d) - E^{(\mathrm{site})}_{\mathrm{NP}} - E^{(\mathrm{site})}_{\mathrm{mol}}$ where $E^{(\mathrm{site})}_{\mathrm{NP}}$ ($E^{(\mathrm{site})}_{\mathrm{mol}}$) is the energy of the system, in its adsorbed configuration, without the molecule (NP). Ticks in the distance axis mark points distances sampled.

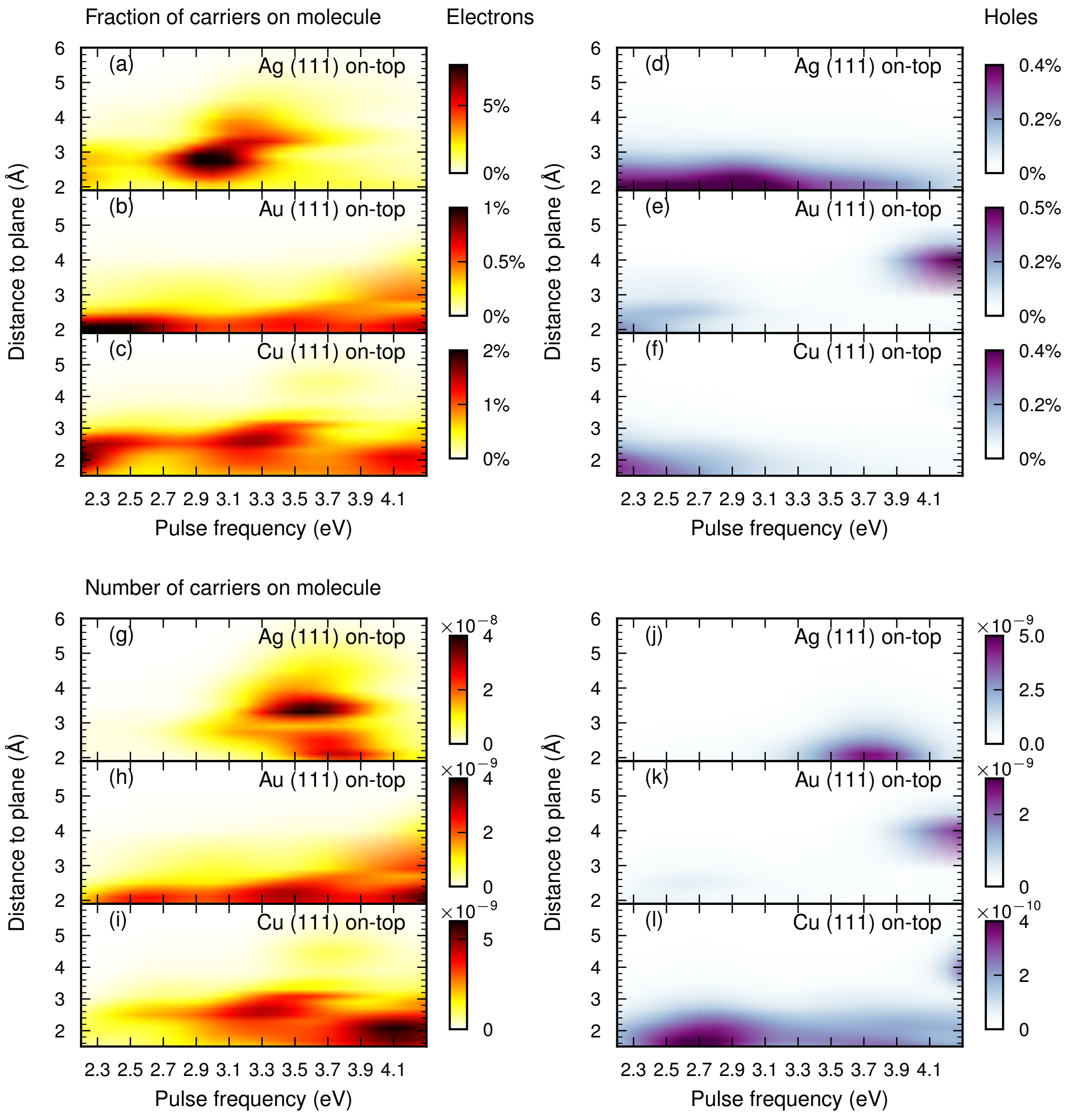


Figure S9: **Pulse-frequency dependence of the electron generation in CO.** The amount of electrons (a-c, g-i) and holes (d-f, j-l) generated on the molecule is expressed as a fraction of carriers (a-f; number of carriers on molecule divided by number of carriers in the combined system) and as a number (g-l).

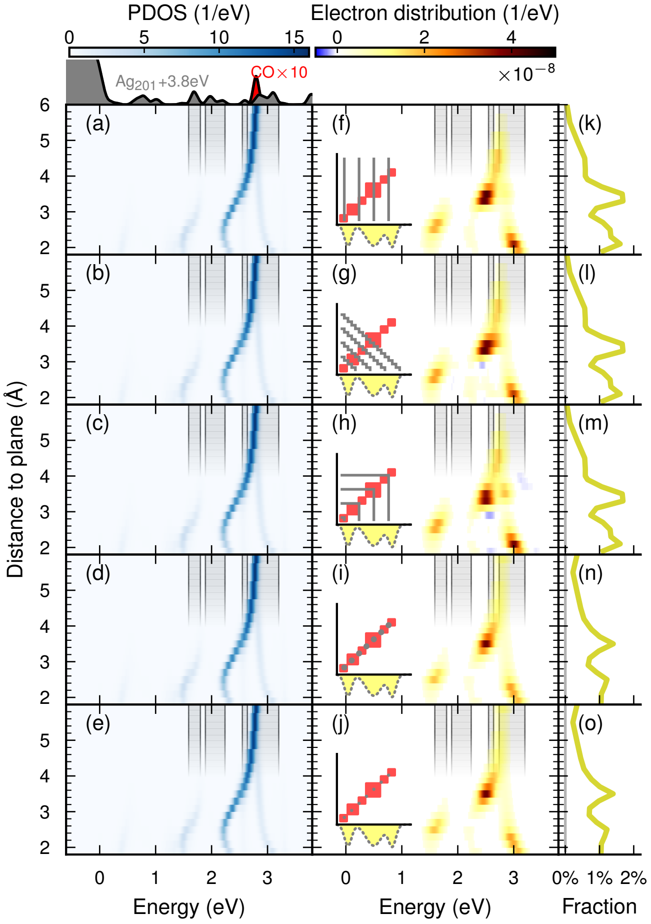


Figure S10: **Alternative formulations of electron distribution in molecule after plasmon decay.** The electron distribution in the molecule is well defined as a sum over unoccupied-unoccupied space $P_{\mathrm{e}}^{(\mathrm{mol})}(\boldsymbol{r}) = \frac{1}{2}\sum_{aa'} M_{aa'} w_{aa'}^{(\mathrm{mol})}$ of the density matrix product $M_{aa'} = \sum_i^{f_i > f_a, f_i > f_{a'}} (q_{ia} q_{ia'} + p_{ia} p_{ia'})$, $w_{aa'}^{(\mathrm{mol})} = \int_{\mathrm{mol}} \psi_a^{(0)}(\boldsymbol{r}) \psi_{a'}^{(0)}(\boldsymbol{r}) \mathrm{d}\boldsymbol{r}$. Simultaneous resolution in energy is not unambiguously defined. (a-e) PDOS on the molecule as a function of distance. All panels are identical. (f-j) Electron distribution expressed as (f) row/column-wise summation $\sum_{aa'} M_{aa'} w_{aa'}^{(\mathrm{mol})} \delta(\varepsilon - \varepsilon_a)$. (g) energy average summation $\sum_{aa'} M_{aa'} w_{aa'}^{(\mathrm{mol})} \delta(\varepsilon - \frac{\varepsilon_a + \varepsilon_{a'}}{2})$. (h) wedge-shape summation $\sum_{aa'} M_{aa'} w_{aa'}^{(\mathrm{mol})} \delta(\varepsilon - \max(\varepsilon_a, \varepsilon_{a'}))$. (i) degenerate-eigenvalue summation $\sum_{aa'} M_{aa'} w_{aa'}^{(\mathrm{mol})} \delta(\varepsilon - \varepsilon_a) \delta(\varepsilon_a - \varepsilon_{a'})$. (j) diagonal-only summation $\sum_{aa'} M_{aa'} w_{aa'}^{(\mathrm{mol})} \delta(\varepsilon - \varepsilon_a) \delta_{aa'}$. Note that between the forms (f-h) the distribution varies only slightly, however with some negative (unphysical) contributions to (g-h). (k-o) Energy integral of the distributions (f-j). For all but the diagonal-only and degenerate eigenvalues summation the end results are identical.

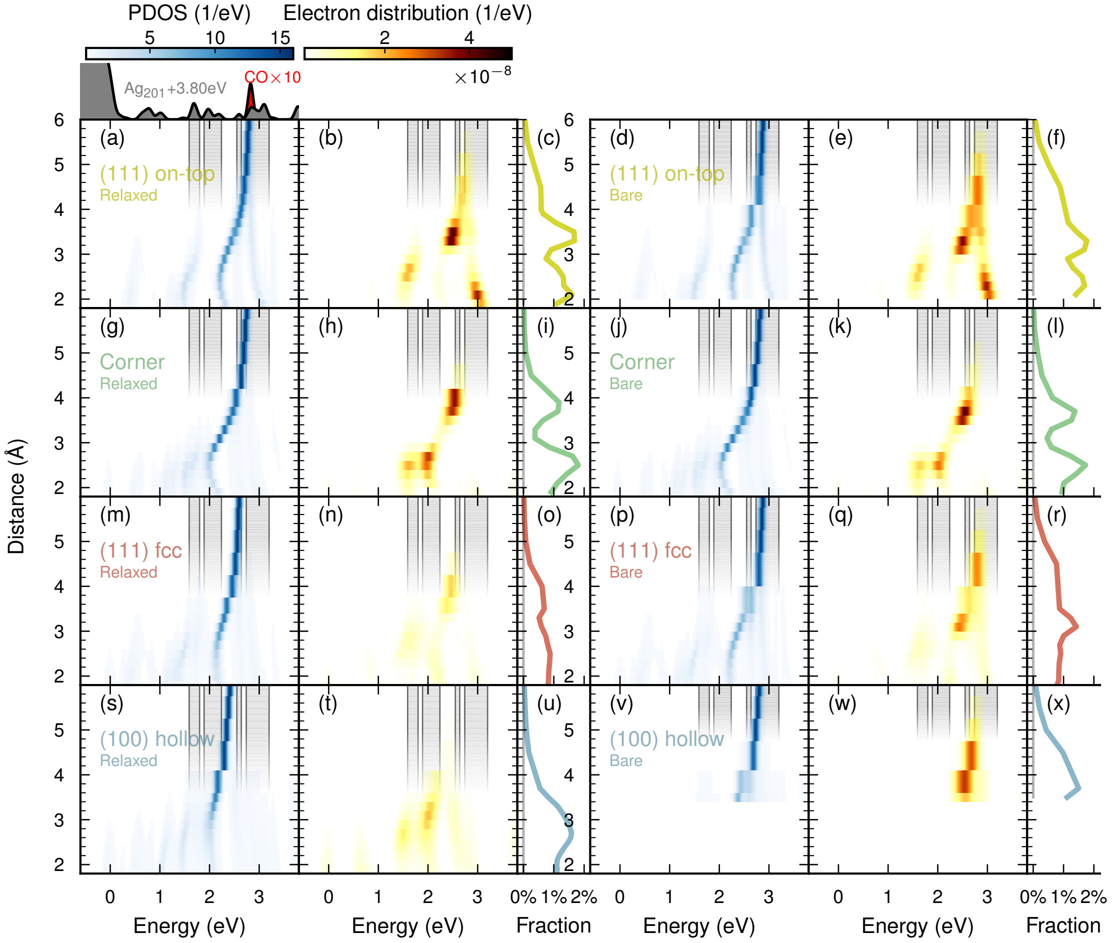


Figure S11: **Level alignment between the projected densities of state of the NP and molecule for $Ag_{201}$.** "Relaxed" refers to the combined system that has been relaxed in the adsorption minimum, and the molecule then shifted. "Bare" refers to the NP being configured as the free NP and the CO with the bond length of the free CO molecule. For the two types of geometries, the molecular PDOS differs primarily by a constant shift of the LUMO orbital energy (most apparent for the (111) fcc and (100) hollow sites). The shift in PDOS changes the resonance condition, and thus the electron distribution on the molecule and fraction of electrons generated on the molecule.

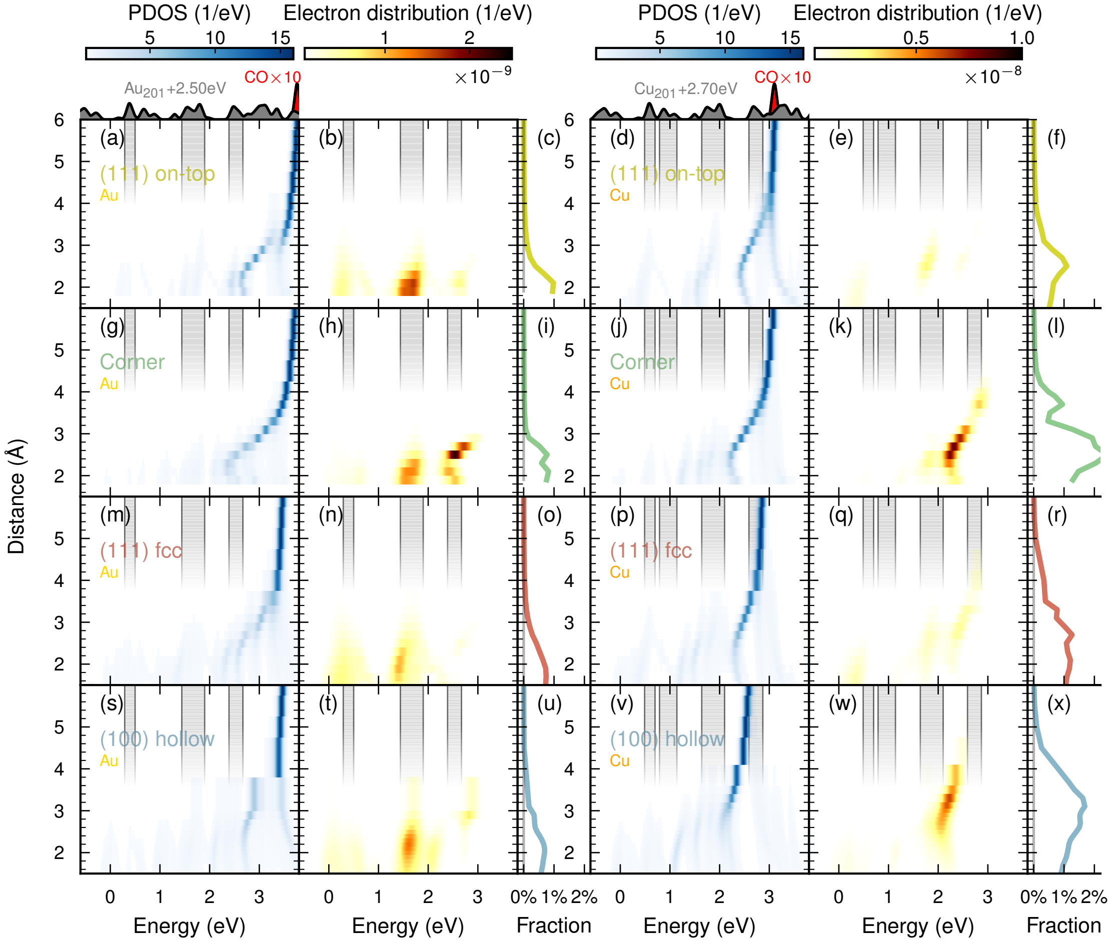


Figure S12: **Level alignment between the projected densities of state of the NP and molecule for $Au_{201}$ and $Cu_{201}$.**

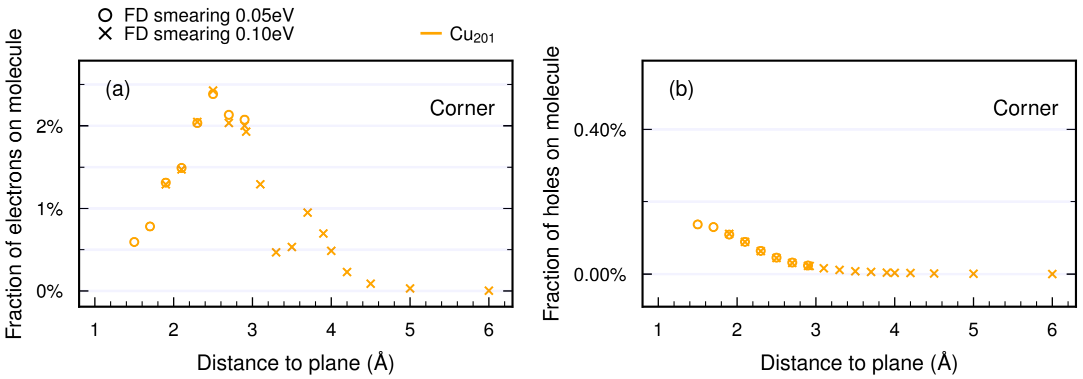


Figure S13: **Carrier generation depending on occupation number smearing.** We compare the fraction of electrons (a) and holes (b) generated on the molecule for the corner site of the $Cu_{201}$ NP. Fermi-Dirac occupation number smearing with the parameters 0.05 eV and 0.1 eV was used. Data is not available at certain distances for the lower value of the smearing parameter (as SCF cycle convergence was difficult to reach with the GLLB-SC xc-functional) but is otherwise in good agreement with the higher parameter value.
